# Supplementary material for: SenseFi: A Library and Benchmark on Deep-Learning-Empowered WiFi Human Sensing
Source: arXiv:2207.07859 source file (2023-02-17)
Supplement: Supplementary file 1 [file 7.appendix.tex]

% \clearpage
% \begin{figure*}[t]
% 	\centering
% 	\includegraphics[width=1\textwidth]{figures/appendix/UT-HAR.pdf}
% 	\caption{The network architectures used in UT-HAR.}\label{fig:ut-har}
% \end{figure*}

% \begin{figure*}[t]
% 	\centering
% 	\includegraphics[width=1\textwidth]{figures/appendix/NTU-HAR.pdf}
% 	\caption{The network architectures used in NTU-Fi HAR.}\label{fig:ntufi-har}
% \end{figure*}
% 
% \begin{figure*}[t]
% 	\centering
% 	\includegraphics[width=1\textwidth]{figures/appendix/NTU-HumanID.pdf}
% 	\caption{The network architectures used in NTU-Fi Human-ID.}\label{fig:ntufi-id}
% \end{figure*}

% \begin{figure*}[t]
% 	\centering
% 	\includegraphics[width=1\textwidth]{figures/appendix/Widar.pdf}
% 	\caption{The network architectures used in Widar.}\label{fig:widar}
% \end{figure*}
